# Supplementary material for: Effect of interfacial oxidation layer in spin pumping experiments on Ni$_{80}$Fe$_{20}$/SrIrO$_3$ heterostructures
Source: arXiv:2005.03727 ancillary file (2020-05-07)
Supplement: Supplementary file 1 [file Supplementary_Material.pdf]

# Supplemental Material: Effect of interfacial oxidation layer in spin pumping experiments on $Ni_{80}Fe_{20}/SrIrO_3$ heterostructures


T.S. Suraj,[2, 3, a)] Manuel Müller,[1] Sarah Gelder,[1] Stephan Geprägs,[1] Matthias Opel,[1] Mathias Weiler,[1, 4] K. Sethupathi,[3] Hans Huebl,[1, 4, 5] Rudolf Gross,[1, 4, 5] M.S. Ramachandra Rao,[2] and Matthias Althammer[1, 4, b)]

[1)] Walther-Meißner-Institut, Bayerische Akademie der Wissenschaften, 85748 Garching, Germany.

[2)]Department of Physics, Nano Functional Materials Technology Center, Material Science Research Center, Indian Institute of Technology Madras (IITM), India 600036.

[3)] Low Temperature Physics Lab, Department of Physics, Indian Institute of Technology Madras (IITM), Chennai, India 600036.

[4)] Physik-Department, Technische Universität München, 85748 Garching, Germany

[5)] Munich Center for Quantum Science and Technology (MCQST), Schellingstr. 4, 80799 München, Germany.



(Dated: 7 May 2020)



a) Electronic email: surajts@physics.iitm.ac.in
b) Electronic email: matthias.althammer@wmi.badw.de

**Sample fabrication**

$SrIrO_3$ (SIO) layer were deposited using pulsed laser deposition (PLD) with a Compex-Pro Excimer Laser operating at 248 nm, under following parameters

| | |
|---|---|
| Laser Fluence | 2 J/cm$^2$ |
| Background oxygen partial pressure ($pO_2$) | 50 µbar |
| Substrate Temperature | 450 °C |
| Substrate to Target distance | 5 cm |
| Repetition rate | 2 Hz |

Subsequently STO//$SrIrO_3$ samples were transferred ex-situ to a sputtering chamber to deposit NbN and $Ni_{80}Fe_{20}$ (NiFe) layers followed by a 3 nm Al capping layer to protect samples from atmospheric oxidation.

**Py deposited on NbN**

The magnetic properties of NiFe are not altered when deposited on NbN. Figure S1 shows the extracted linewidth from BBFMR of a 15 nm Py layer grown on 16 nm NbN layer at T=300 K. We extract a Gilbert damping $\alpha = 6.6 \times 10^{-3}$, which exactly matches the bulk damping of NiFe.[1,2]

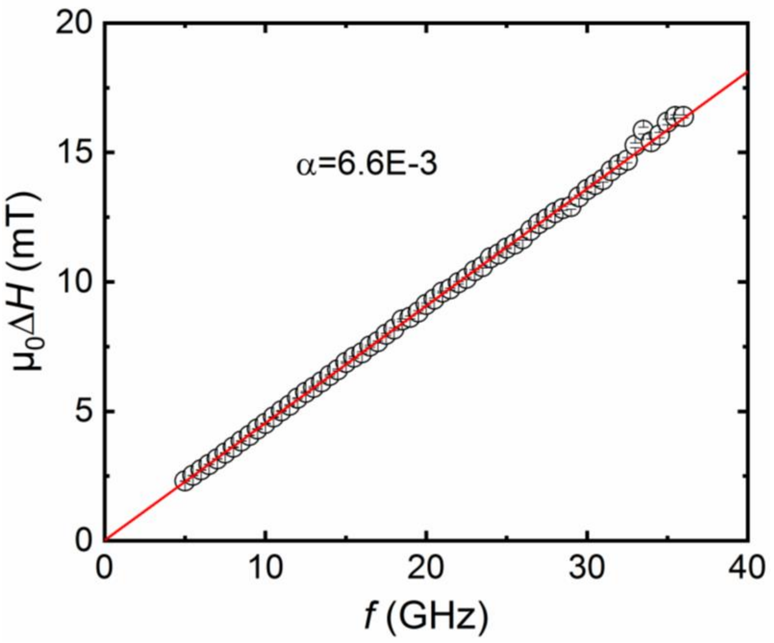


Figure S1: The extracted linewidth as a function of applied microwave frequency at room temperature for a NiFe(16 nm)/NbN(15 nm) sample. The Gilbert damping parameter α is extracted by fitting Eq. (S1) (red line).

## Temperature dependent changes in Linewidth

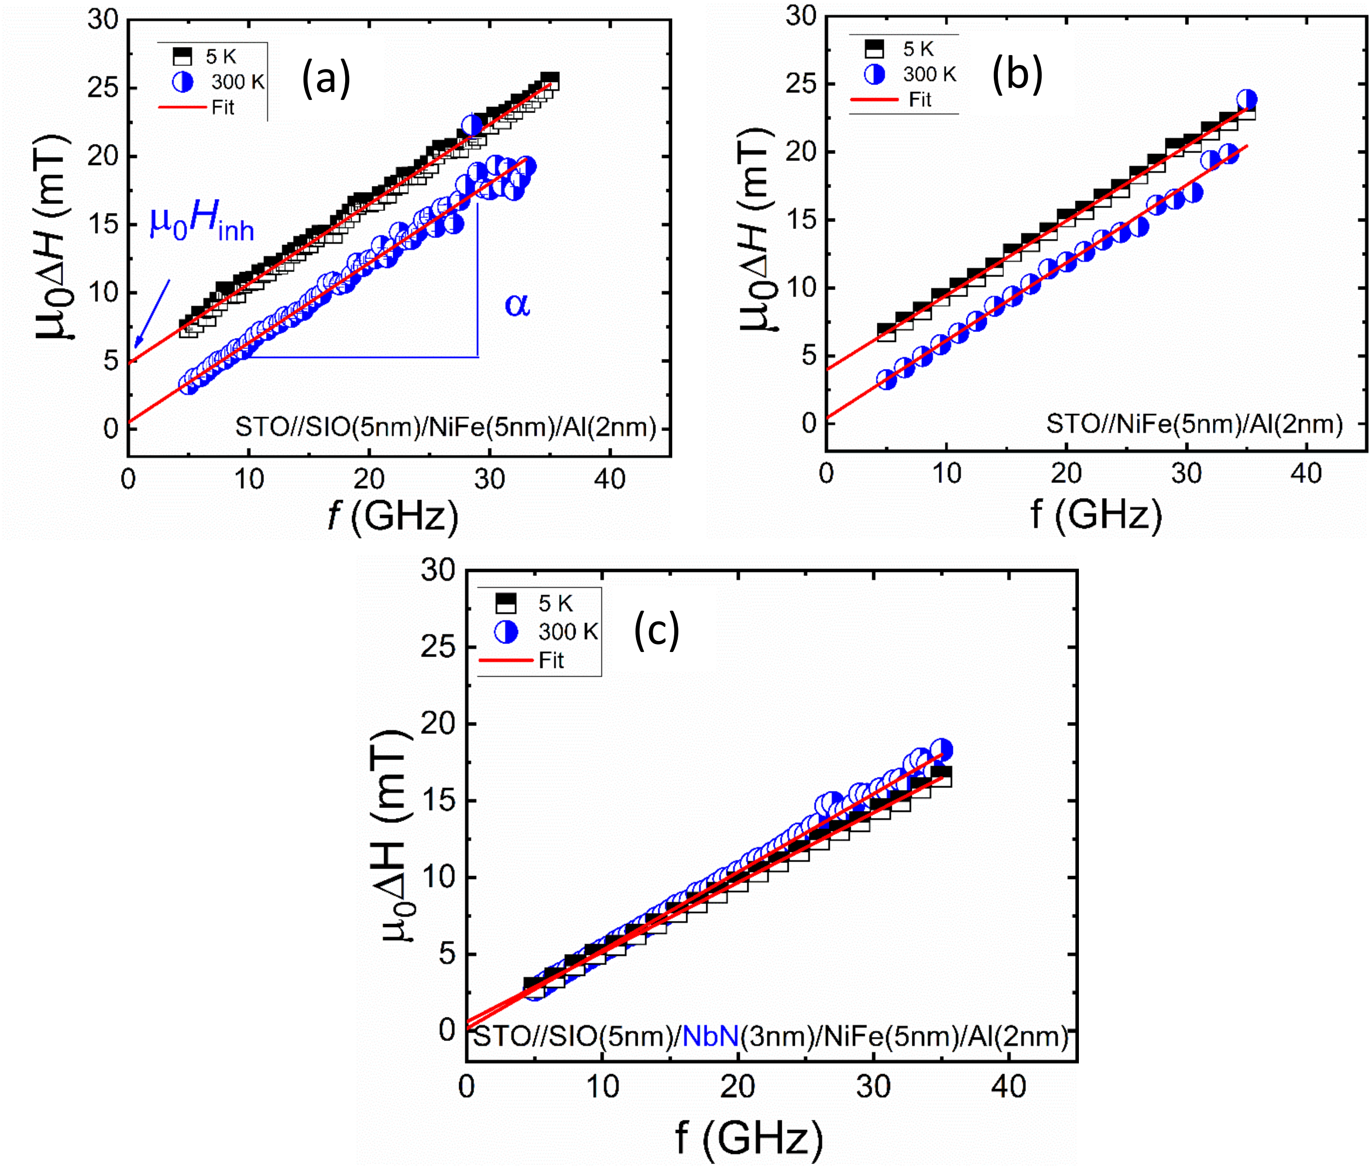


Figure S2: The extracted linewidth as a function of applied microwave frequency at 5 K and 300 K for STO//SIO/NiFe(5 nm)/Al(2 nm) (a), STO//NiFe(5 nm)/Al(2 nm) (b) and STO//SIO/NbN(3 nm)/NiFe(5 nm)/Al(2 nm) (c) sample. The Gilbert damping parameter (α) is extracted by fitting Eq. (S1) (red lines).

Linewidth extracted from BBFMR measurements at 5 K and 300 K for STO//SIO/NiFe/Al, STO//NiFe/Al and STO//SIO/NbN/NiFe/Al are fitted using. (Fig S2)

$$\mu_0 \Delta H = \mu_0 H_{inh} + 2\frac{2\pi f \alpha}{\gamma}, \quad \text{(S1)}$$

With ‘$\gamma$’ the gyromagnetic ratio. The Gilbert damping ‘α’ and inhomogeneous line broadening $\mu_0 H_{\mathrm{inh}}$ are extracted from slope and intercept, respectively. The extracted α and $\mu_0 H_{inh}$ at different temperatures are shown in Fig. 3a and 3c in the main text.

**<u>Temperature dependent changes in resonance field</u>**

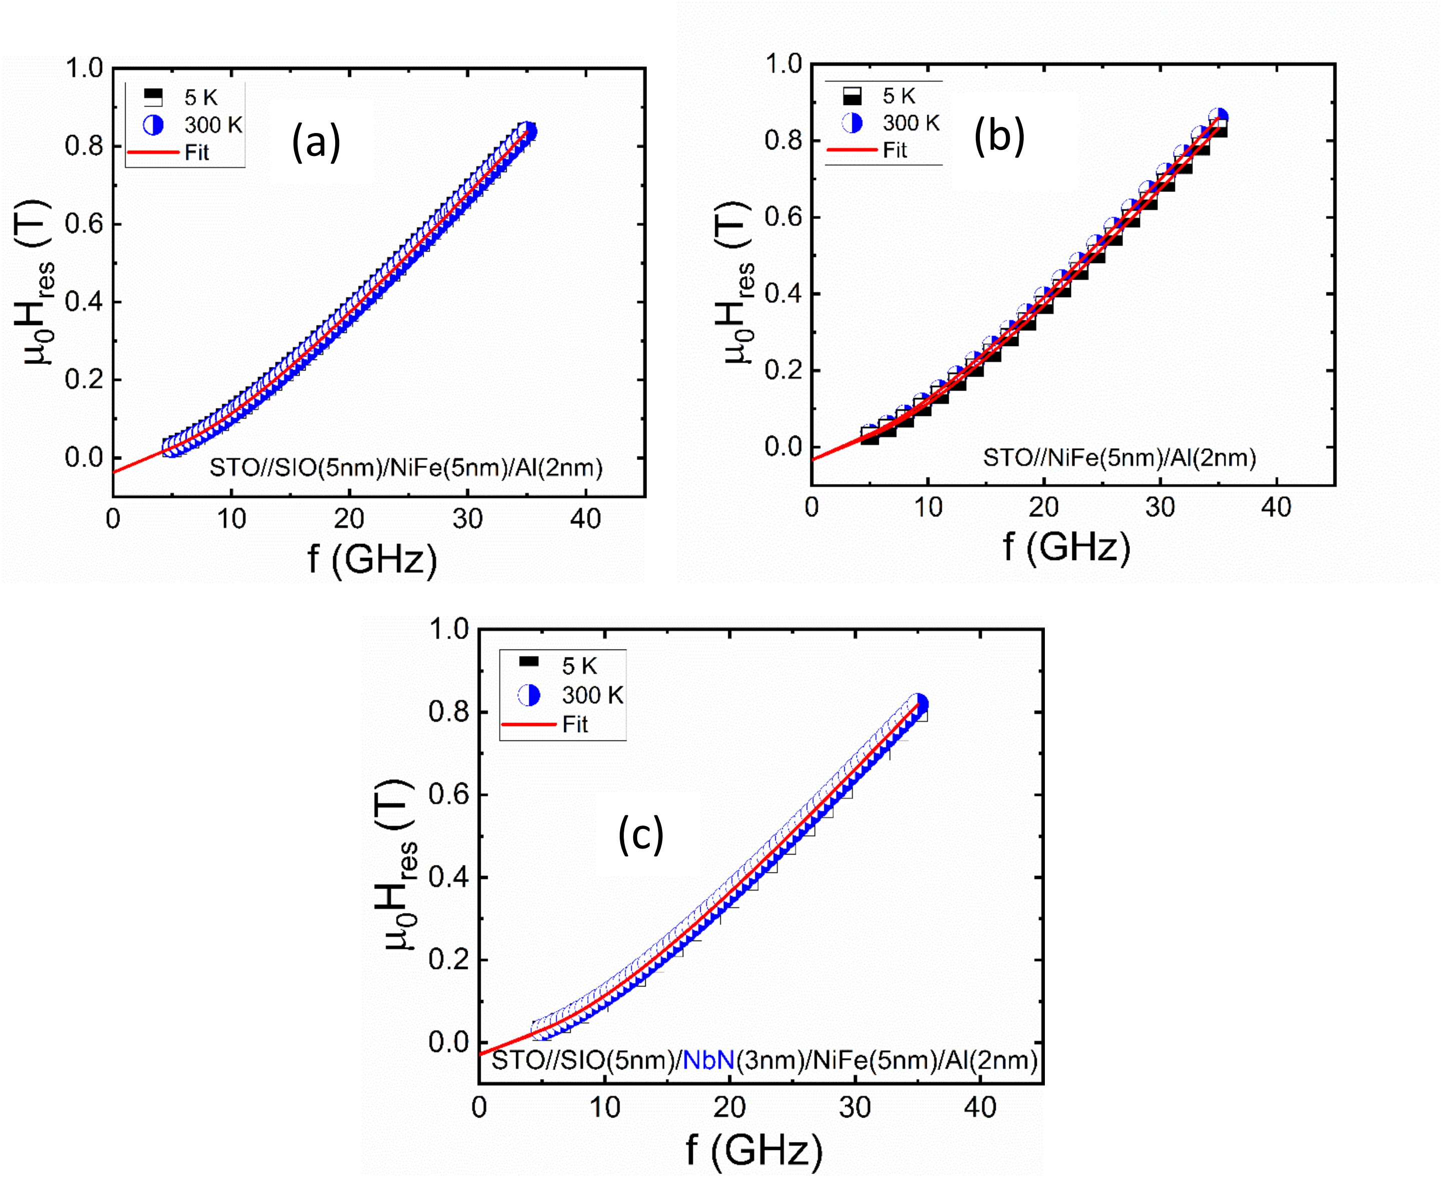


Figure S3: The resonance field as a function of applied microwave frequency at 5 K and 300 K for STO//SIO/NiFe(5 nm)/Al(2 nm) (a), STO//NiFe(5 nm)/Al(2 nm) (b) and STO//SIO/NbN(3 nm)/NiFe(5 nm)/Al(2 nm) (c) sample. The anisotropy field and effective magnetization are extracted by fitting the data to Eq.(S2) (red lines).

Similarly, resonance fields extracted from BBFMR measurements were fitted using Kittel equation[3]

$$\mu_0 H_{\mathrm{res}} = -\mu_0 H_{\mathrm{ani}} - \frac{\mu_0 M_{\mathrm{eff}}}{2} + \sqrt{\left(\frac{\mu_0 M_{\mathrm{eff}}}{2}\right)^2 + \left(\frac{2\pi f}{\gamma}\right)^2} \qquad \text{(S2)}$$

For the in-plane magnetization case, we can extract from the frequency dependence of $\mu_0 H_{\mathrm{res}}$ the effective magnetization $M_{\mathrm{eff}}$ and the in-plane anisotropy field $\mu_0 H_{\mathrm{ani}}$. The $\mu_0 H_{\mathrm{res}}$ and $\mu_0 H_{\mathrm{ani}}$ values at different temperatures are shown in Fig.3b and 3d in the main text.

**Inhomogeneous line broadening in OOP geometry**

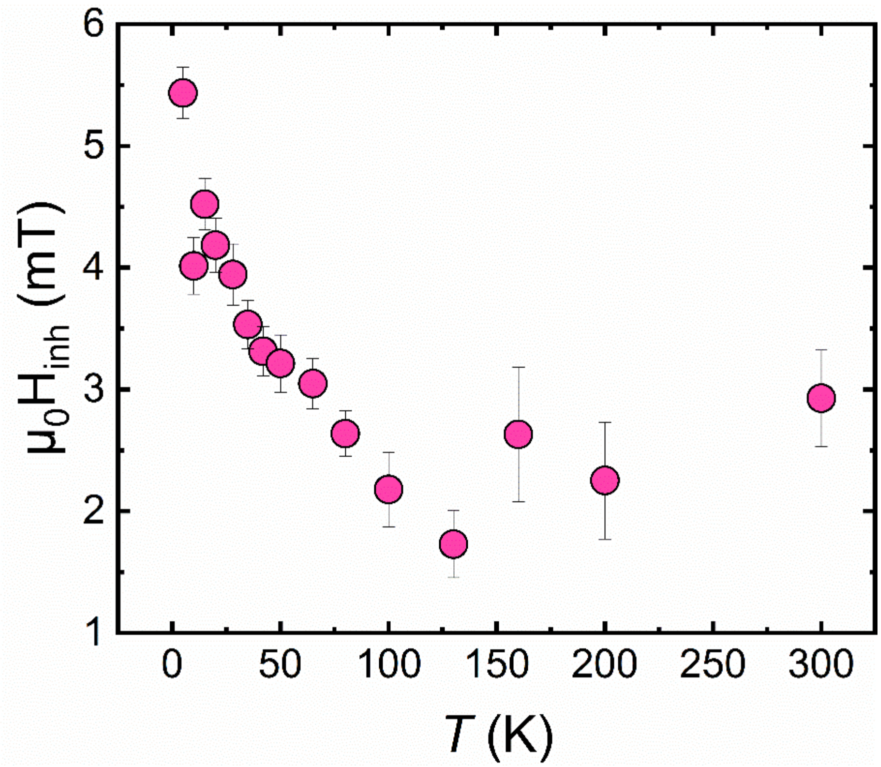


Figure S4: The inhomogeneous line broadening $\mu_0 H_{\mathrm{inh}}$ for NiFe(7 nm)/SIO(5 nm) as a function of temperature in out of plane geometry.

To rule out two magnon scattering as a possible source for the increase of $\mu_0 H_{\mathrm{inh}}$ towards low temperature we show inhomogeneous line broadening recorded in the out-of plane geometry for a NiFe(7 nm)/SIO(5 nm) sample. In this geometry, two magnon scattering is absent and the similar increase of $\mu_0 H_{\mathrm{inh}}$ towards low temperature rules out two magnon scattering as the dominant source of the observed changes in the main text.

## Spin mixing conductance

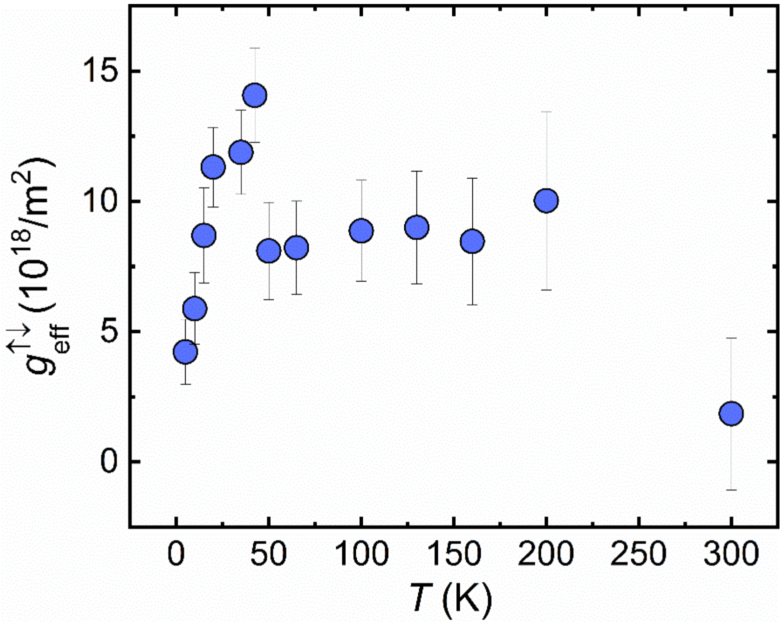


Figure S5: The extrapolated spin mixing conductance as a function of temperature by comparing $\alpha$ of a NiFe(7 nm)/SIO(5 nm) and NiFe(5 nm)/SIO(5 nm) by using Eq. (S4).

We employ a linear fit of the form

$$\alpha = \alpha_0 + \alpha_{SP}\left(\frac{1}{d_{FM}}\right) \qquad \text{(S3)}$$

to extract spin pumping contribution of Gilbert damping . Where the bulk Gilbert damping, $\alpha_0$= 6.44 x $10^{-3} \pm 8$ x $10^{-5}$ corresponds well to literature [5,6,7,8], while the slope $\alpha_{SP}$ can be employed to quantify the effective spin mixing conductance $g_{eff}^{\uparrow\downarrow}$ by linearly fitting

$$\alpha_0 + \alpha_{SP} = \alpha_0 + 2\frac{\gamma\hbar g_{eff}^{\uparrow\downarrow}}{4\pi M_s}\left(\frac{1}{d_{FM}}\right) \quad (S4)$$

at different temperatures. The temperature dependence saturation magnetization $\mu_0 M_s$ was modeled by extrapolating the bulk value for $\mu_0 M_s = 0.98\ \text{T} = 1.24\ \text{T}\left[1-\left(\frac{300\ \text{K}}{843\ \text{K}}\right)^{3/2}\right]$ from our layer thickness series at the temperature $T$ = 300 K using Bloch's law [8]

$$\mu_0 M_s = 1.24\ \text{T}\left(1-\left(\frac{T}{T_C}\right)^{3/2}\right) \qquad (5)$$

The Curie temperature $T_C$ = 843 K was chosen for NiFe.[4] The spin mixing conductance shows a maximum near 50 K, which is attributed to enhanced spin pumping near the Néel temperature of $NiFeO_x$.

**Interface anisotropy in NiFe/SIO bilayers**

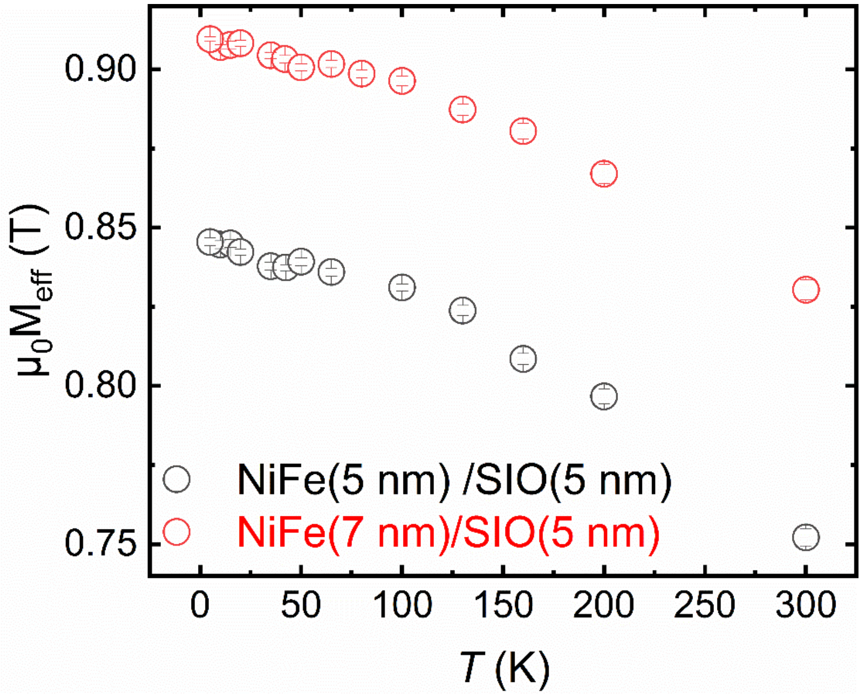


Figure S6: The extracted effective magnetization for NiFe(5 nm)/ SIO(5 nm) and NiFe(7 nm)/ SIO(5 nm) sample as a function of temperature.

A comparison in the effective magnetization $\mu_0 M_{\text{eff}}$ as function of temperature for two NiFe/SIO-samples with different thickness. The disparity in their $\mu_0 M_{\text{eff}}$ is evidence of an interface anisotropy in these samples.[9]

**References**


1. J. E. Gómez, B. Zerai Tedlla, N. R. Álvarez, G. Alejandro, E. Goovaerts, and A. Butera, "Spin transport parameters in $Ni_{80}Fe_{20}$/Ru and $Ni_{80}Fe_{20}$/Ta bilayers," *Phys. Rev. B* 90, 184401 (2014).
2. A. J. Berger, E. R. J. Edwards, H. T. Nembach, A. D. Karenowska,, M.Weiler, and T. J. Silva, "Inductive detection of field like and damping like ac inverse spin-orbit torques in ferromagnet/normal-metal bilayers," *Phys.Rev. B* 97, 094407 (2018).
3. C. Kittel, "On the theory of ferromagnetic resonance absorption," Phys. Rev. 73, 155–161 (1948).
4. W. Bailey, P. Kabos, F. Mancoff, and S. Russek, IEEE Transactions on Magnetics 37 (4), 1749 (2001).
5. J. O. Rantschler, B. B. Maranville, J. J. Mallett, P. Chen, R. D. McMichael, and W. F. Egelhoff, IEEE Transactions on Magnetics 41 (10), 3523 (2005).
6. C. Luo, Z. Feng, Y. Fu, W. Zhang, P. K. J. Wong, Z. X. Kou, Y. Zhai, H. F. Ding, M. Farle, J. Du, and H. R. Zhai, Physical Review B 89 (18), 184412 (2014).

7. A. Ghosh, J. F. Sierra, S. Auffret, U. Ebels, and W. E. Bailey, Applied Physics Letters 98 (5), 052508 (2011).
8. Ashcroft, Neil W.; Mermin, N. David (1976). Solid State Physics. Holt, Rinehart and Winston. ISBN 0-03-083993-9.
9. J. Michael. D. Coey. Magnetism and Magnetic Materials. Cambridge, 2010.
